# Supplementary material for: PTR: A Benchmark for Part-based Conceptual, Relational, and Physical Reasoning
Source: arXiv:2112.05136 source file (2021-12-09)
Supplement: Supplementary file 1 [file supp_examples.pdf]

## Concept

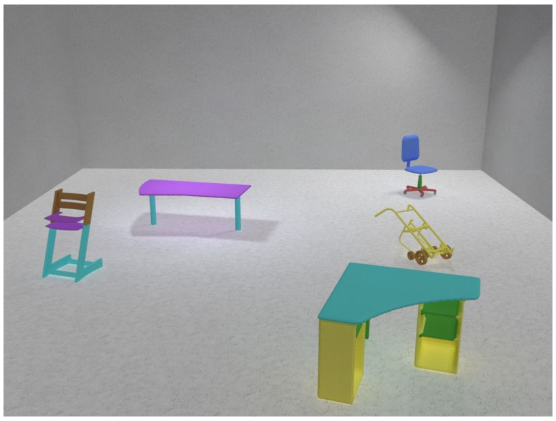

**Q:** *How many things with wheels are there?*
**A:** *2*
**Q-type:** *count_object*

**Q:** *Are there any objects with two cyan legs?*
**A:** *Yes*
**Q-type:** *exist_object*

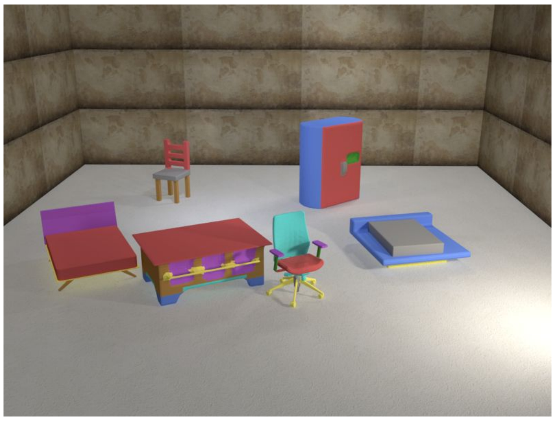

**Q:** *How many legs does the object with one central support have?*
**A:** *5*
**Q-type:** *count_part*

**Q:** *What is the color of the sleep area of the bed with brown legs?*
**A:** *Red*
**Q-type:** *query_part*

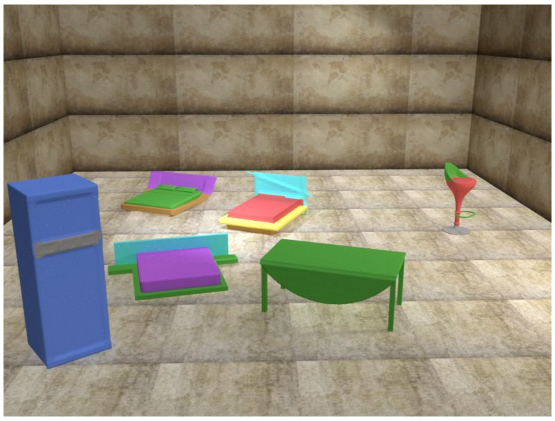

**Q:** *How many beds with cyan back are there?*
**A:** *2*
**Q-type:** *count_object*

**Q:** *What is the category of the thing with legs?*
**A:** *Table*
**Q-type:** *query_object*

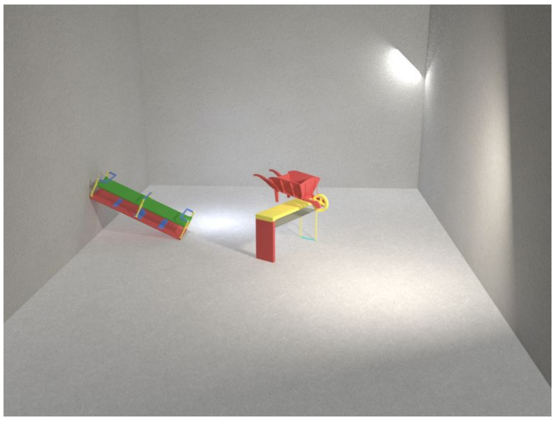

**Q:** *How many tables with shelves are there?*
**A:** *2*
**Q-type:** *count_object*

**Q:** *Are there any objects with yellow legs?*
**A:** *Yes*
**Q-type:** *exist_object*

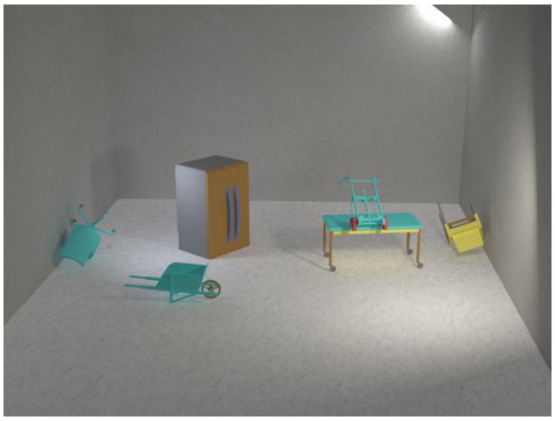

**Q:** *What is the color of the top of the table with brown legs?*
**A:** *cyan*
**Q-type:** *query_part*

**Q:** *How many doors does the refrigerator have?*
**A:** *2*
**Q-type:** *count_part*

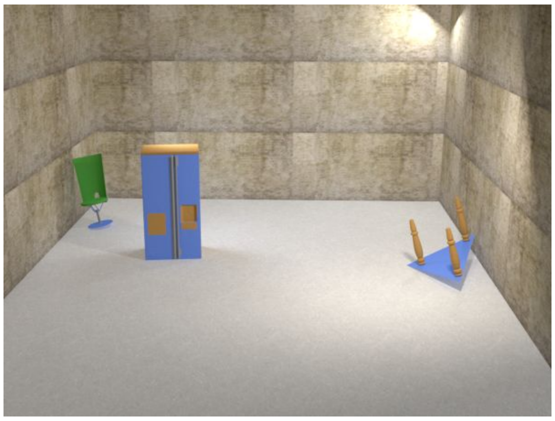

**Q:** *What is the color of the pedestal of the chair?*
**A:** *Blue*
**Q-type:** *query_part*

**Q:** *How many legs does the table have?*
**A:** *3*
**Q-type:** *count_part*

## Relation

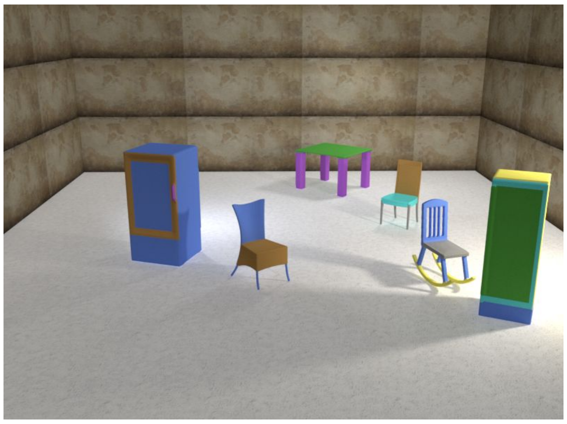

**Q:** *What is the number of the visible legs of the thing that has the same color of back as the chair with one gray seat?*
**A:** *3*
**Q-type:** *same_relate*

**Q:** *Are the object with purple legs and the object with gray legs of the same category?*
**A:** *No*
**Q-type:** *same_relate*

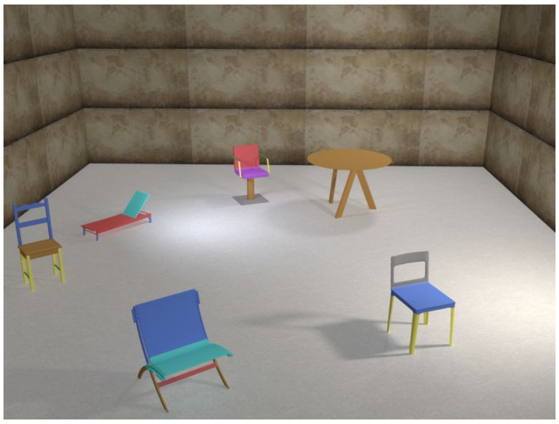

**Q:** *What is the category of the object with brown legs that is on the right side of the chair with a pedestal?*
**A:** *Table*
**Q-type:** *spatial_relationship*

**Q:** *What is the category of the green part of the object with four visible legs that is on the left side of the chair with two arm vertical bars?*
**A:** *Leg bar*
**Q-type:** *spatial_relationship*

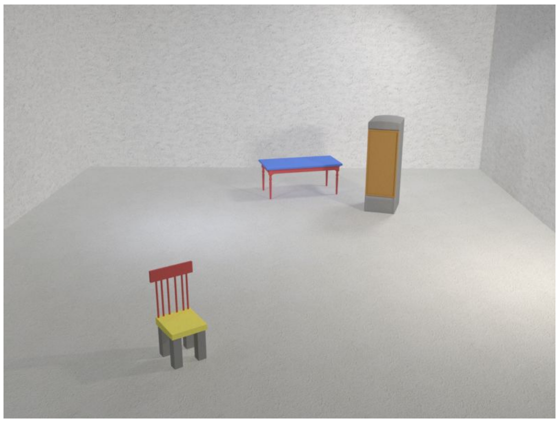

**Q:** *Is there a part in the chair that can be considered a line, and is parallel to the brown part of the refrigerator?*
**A:** *No*
**Q-type:** *geometric_relationship*

**Q:** *What is the color of the part in the chair that can be considered a plane, and is perpendicular to the brown part of the refrigerator?*
**A:** *Yellow*
**Q-type:** *geometric_relationship*

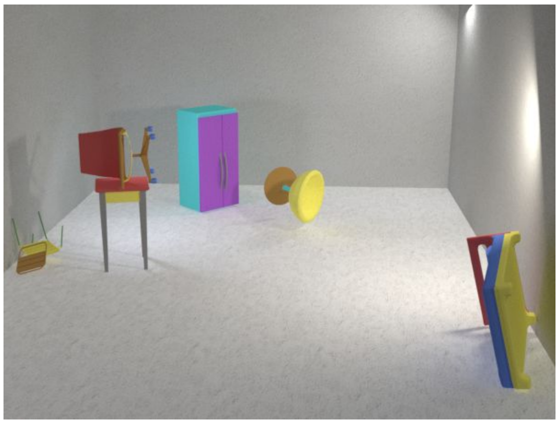

**Q:** *What is the color of the legs of the thing that has the same color of back as the bed?*
**A:** *Brown*
**Q-type:** *same_relate*

**Q:** *Are the body of the refrigerator, and the central support of the chair with pedestal of the same color?*
**A:** *Yes*
**Q-type:** *same_relate*

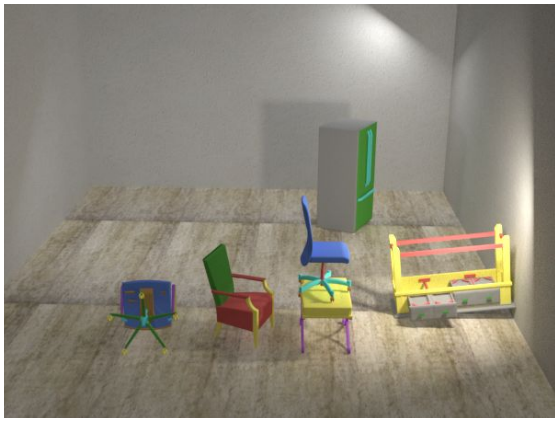

**Q:** *How many things with legs are in front of the refrigerator?*
**A:** *5*
**Q-type:** *spatial_relationship*

**Q:** *What is the color of the leg bars of the thing with yellow legs that is to the right of the table with yellow top?*
**A:** *Red*
**Q-type:** *spatial_relationship*

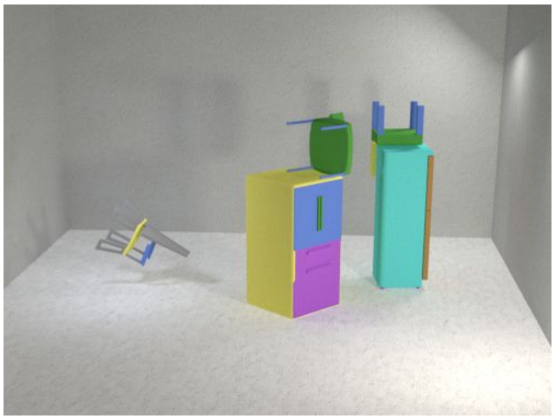

**Q:** *How many parts in the chair with green seat can be considered as lines, and are perpendicular to the blue part of the refrigerator with blue body?*
**A:** *4*
**Q-type:** *geometric_relationship*

**Q:** *Is there a part in the chair with gray legs that can be considered a plane, and is perpendicular to the blue part of the refrigerator?*
**A:** *No*
**Q-type:** *geometric_relationship*

## Analogy

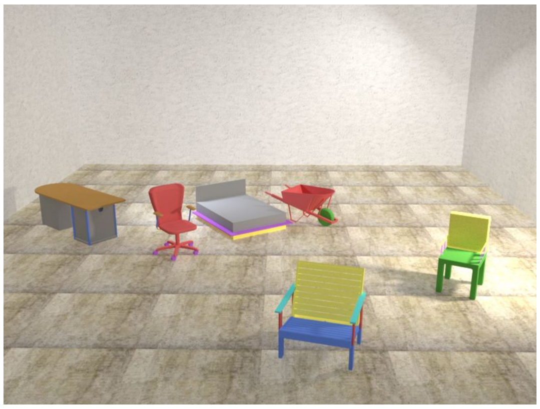

**Q:** *The thing with five legs has certain positional relation to the object with blue seat. By analogy, how many objects does the bed have the same positional relation to ?*
**A:** *2*
**Q-type:** *positional analogy*

**Q:** *The cart has certain positional relation to the chair with central support. By analogy, is there an object that the chair with green seat has the same positional relation to?*
**A:** *Yes*
**Q-type:** *positional_analogy*

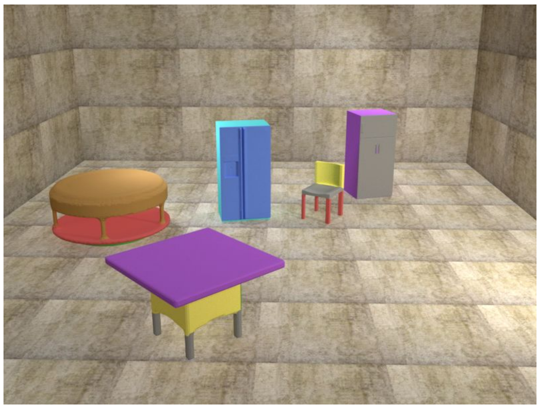

**Q:** *The purple part of the table with three gray legs has certain geometric relation to the red part of the table with one brown top. by analogy, the blue part of the refrigerator with cyan body has the same geometric to the part of which color in the refrigerator with purple body?*
**A:** *gray*
**Q-type:** *geometric_analogy*

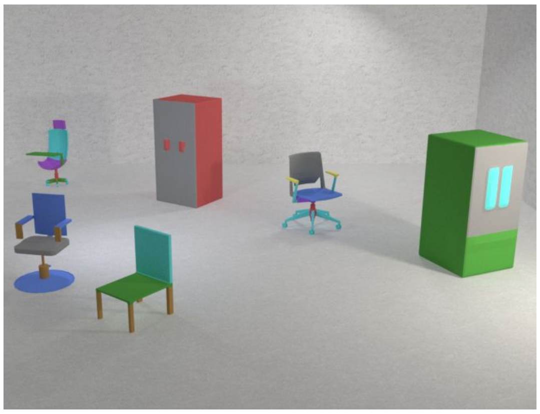

**Q:** *The yellow parts of the chair with gray back have certain geometric relation to the gray part of the refrigerator with green body. By analogy, the brown parts of the chair with green seat have the same geometric relation to a part of what color in the chair with cyan legs?*
**A:** *Blue*
**Q-type:** *geometric_analogy*

## Arithmetic

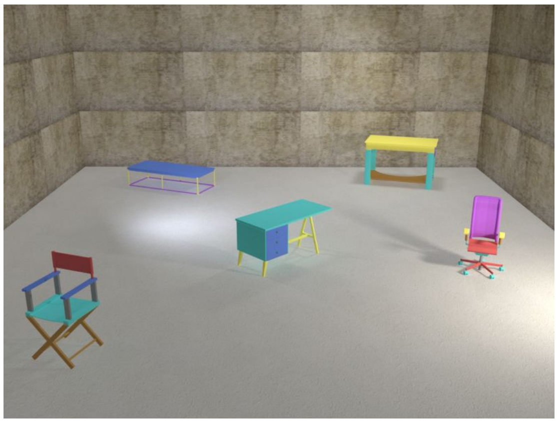

**Q:** *What is the sum of the legs in the table with blue top, and the number of drawers in the table with cyan top?*
**A:** *9*
**Q-type:** *sum-minus*

**Q:** *What is the number of arm vertical bars in the chair with brown legs, subtracted by the number of drawers in the table with cyan top?*
**A:** *1*
**Q-type:** *sum-minus*

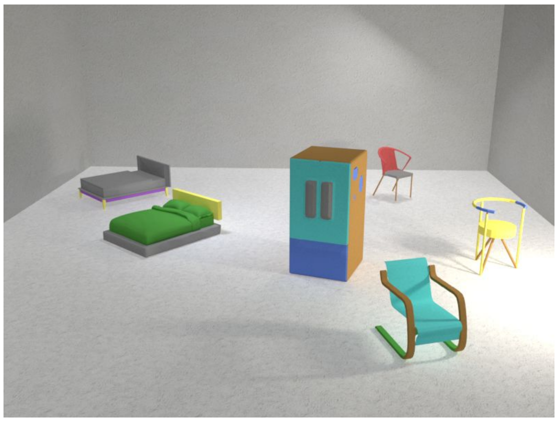

**Q:** *Are there an equal number of doors in the refrigerator, and leg bars in the chair with cyan seat?*
**A:** *Yes*
**Q-type:** *compare-integer*

**Q:** *Are there fewer legs in the chair with gray seat, than legs in the chair with yellow seat?*
**A:** *No*
**Q-type:** *compare-integer*

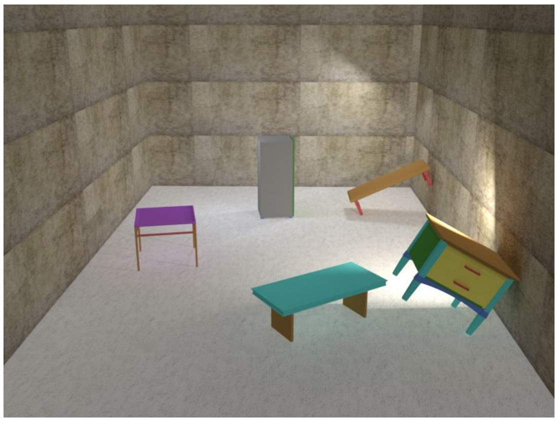

**Q:** *Are there fewer legs in the table with purple top, than drawers in the table with cyan legs?*
**A:** *No*
**Q-type:** *compare-integer*

**Q:** *What is the number of drawers in the table with cyan legs, subtracted from the number of legs in the table with purple top?*
**A:** *2*
**Q-type:** *sum-minus*

**Physics**

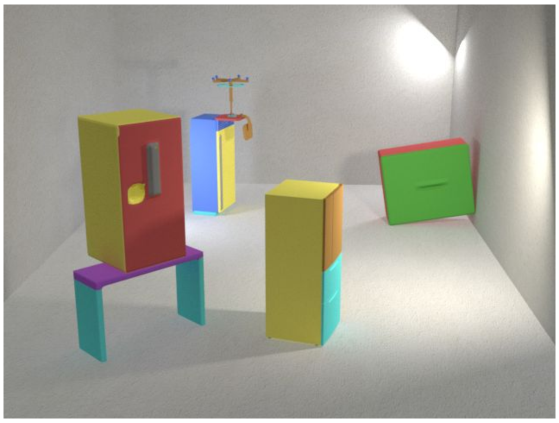

**Q:** *Is the chair stable?*
**A:** *No*
**Q-type:** *stability*

**Q:** *Towards which direction should the chair move to become stable?*
**A:** *To left*
**Q-type:** *possible changes*

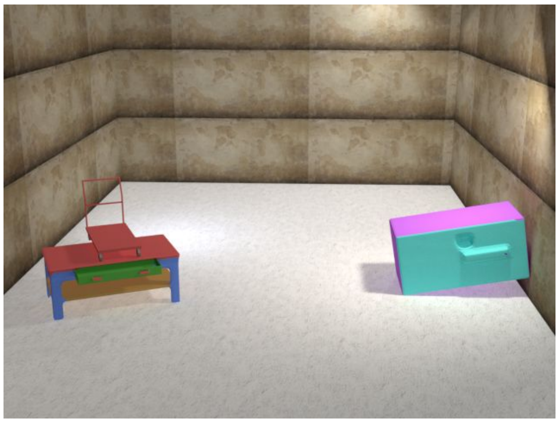

**Q:** *How many objects are stable?*
**A:** 1
**Q-type:** *stability*

**Q:** *Can moving front makes the cart stable?*
**A:** *no*
**Q-type:** *possible changes*

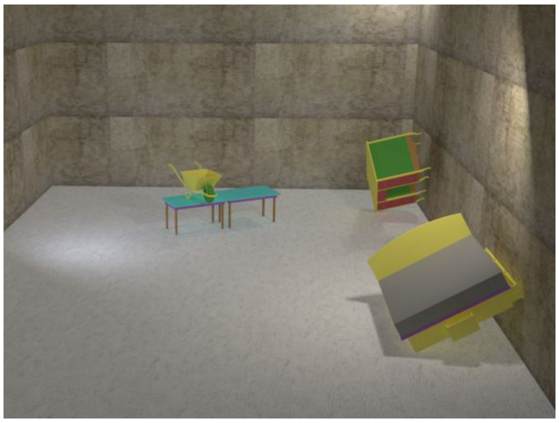

**Q:***Is the table* with *yellow top stable?*
**A:** *No*
**Q-type:** *stability*

**Q:** *Is the bed stable?*
**A:** *Yes*
**Q-type:** *stability*
