# Supplementary material for: PTR: A Benchmark for Part-based Conceptual, Relational, and Physical Reasoning
Source: arXiv:2112.05136 source file (2021-12-09)
Supplement: Supplementary file 2 [file supp_examples-v2.pdf]

## Concept

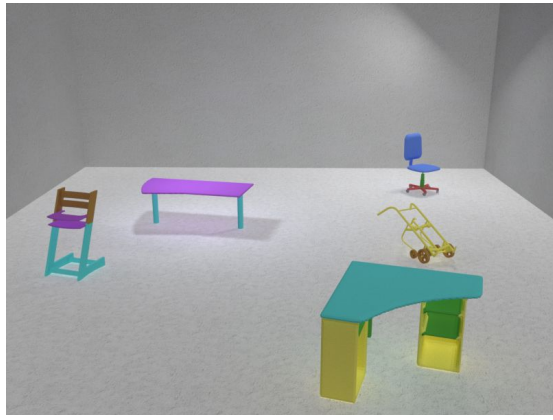

**Q:** How many things with *wheels* are there?

**A:** 2

**Q-type:** count\_object

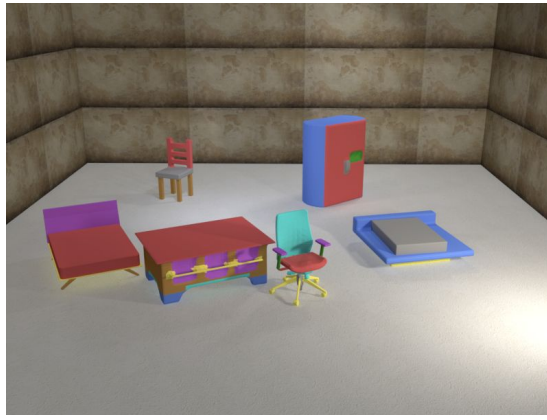

**Q:** How many *legs* does the object with one *central support* have?

**A:** 5

**Q-type:** count\_part

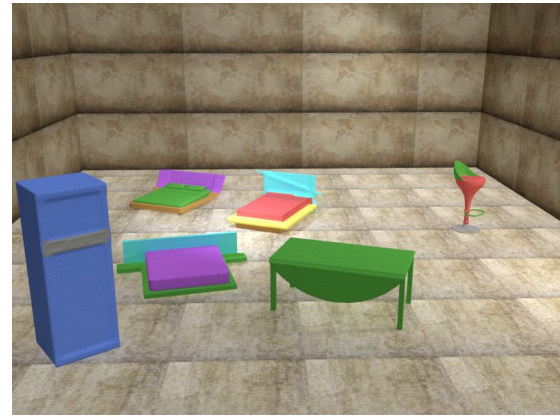

**Q:** How many *beds* with *cyan back* are there?

**A:** 2

**Q-type:** count\_object

**Q:** Are there any objects with two *cyan legs*?

**A:** Yes

**Q-type:** exist\_object

**Q:** What is the color of the *sleep area* of the *bed* with *brown legs*?

**A:** Red

**Q-type:** query\_part

**Q:** What is the *category* of the thing with *legs*?

**A:** Table

**Q-type:** query\_object

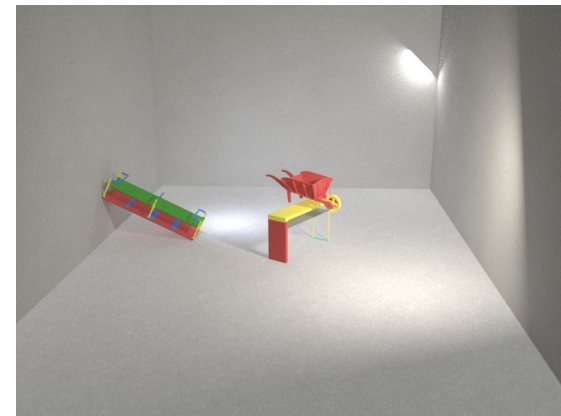

**Q:** How many *tables* with *shelves* are there?

**A:** 2

**Q-type:** count\_object

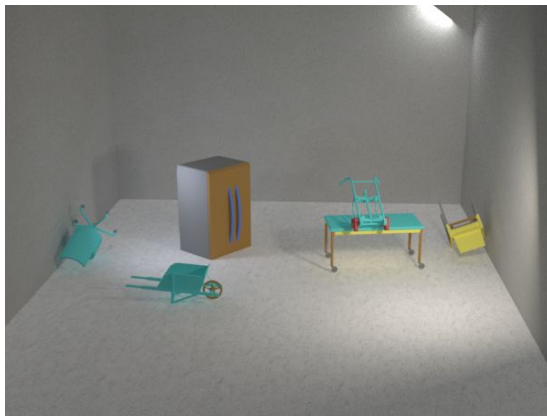

**Q:** What is the *color* of the *top* of the *table* with *brown legs*?

**A:** cyan

**Q-type:** query\_part

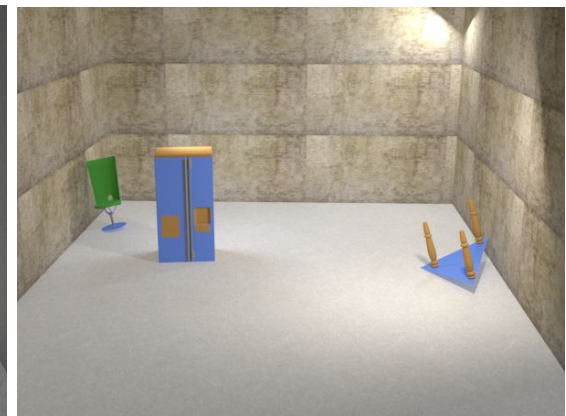

**Q:** What is the *color* of the *pedestal* of the *chair*?

**A:** Blue

**Q-type:** query\_part

**Q:** Are there any objects with *yellow legs*?

**A:** Yes

**Q-type:** exist\_object

**Q:** How many *doors* does the *refrigerator* have?

**A:** 2

**Q-type:** count\_part

**Q:** How many *legs* does the *table* have?

**A:** 3

**Q-type:** count\_part

# Relation

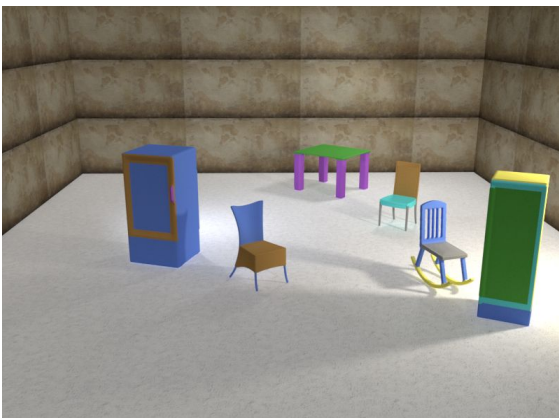

**Q:** What is the number of the visible *legs* of the thing that has the same *color of back* as the *chair* with one *gray seat*?

**A:** 3

**Q-type:** *same\_relate*

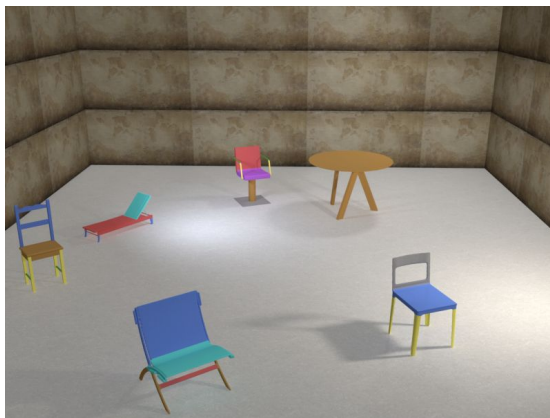

**Q:** What is the *category* of the object with *brown legs* that is on the right side of the *chair* with a *pedestal*?

**A:** *Table*

**Q-type:** *spatial\_relationship*

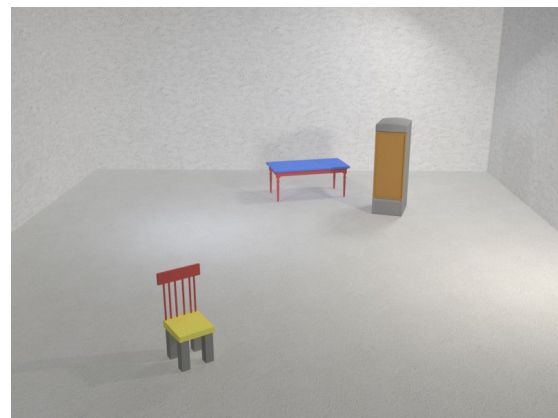

**Q:** Is there a part in the *chair* that *can be considered a line*, and is *parallel* to the *brown* part of the *refrigerator*?

**A:** No

**Q-type:** *geometric\_relationship*

**Q:** Are the object with *purple legs* and the object with *gray legs* of the same *category*?

**A:** No

**Q-type:** *same\_relate*

**Q:** What is the *category* of the *green* part of the object with four visible *legs* that is on the left side of the *chair* with two *arm vertical bars*?

**A:** *Leg bar*

**Q-type:** *spatial\_relationship*

**Q:** What is the *color* of the part in the *chair* that can be considered a *plane*, and is *perpendicular* to the *brown* part of the *refrigerator*?

**A:** *Yellow*

**Q-type:** *geometric\_relationship*

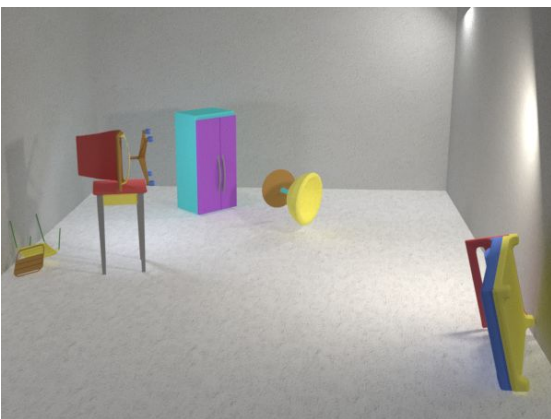

**Q:** What is the *color* of the *legs* of the thing that has the same *color of back* as the *bed*?

**A:** *Brown*

**Q-type:** *same\_relate*

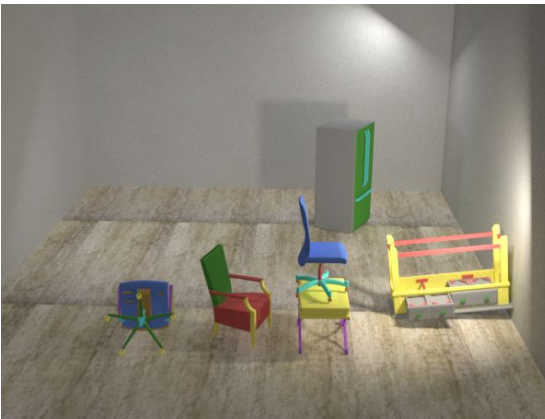

**Q:** How many things with *legs* are in front of the *refrigerator*?

**A:** 5

**Q-type:** *spatial\_relationship*

**Q:** Are the *body* of the *refrigerator*, and the *central support* of the *chair* with *pedestal* of the same *color*?

**A:** Yes

**Q-type:** *same\_relate*

**Q:** What is the *color* of the *leg bars* of the thing with *yellow legs* that is to the right of the *table* with *yellow top*?

**A:** *Red*

**Q-type:** *spatial\_relationship*

## Analogy

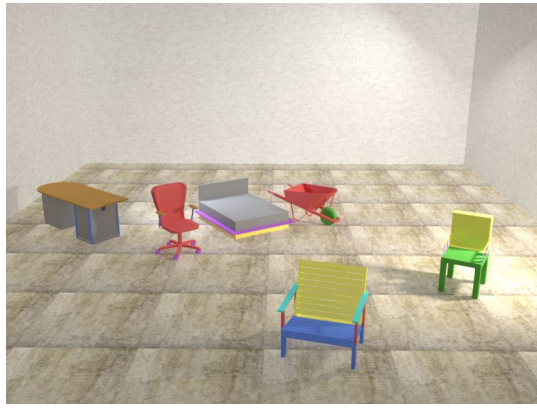

**Q:** The thing with five *legs* has certain positional relation to the object with *blue seat*. By analogy, how many objects does the *bed* have the same positional relation to ?

**A:** 2

**Q-type:** positional analogy

**Q:** The *cart* has certain positional relation to the *chair* with *central support*. By analogy, is there an object that the *chair* with *green seat* has the same positional relation to?

**A:** Yes

**Q-type:** positional\_analogy

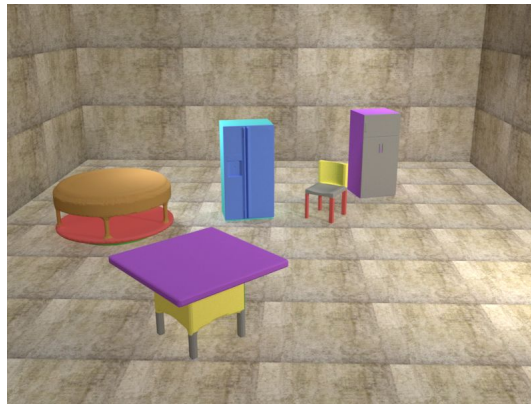

**Q:** The *purple* part of the *table* with three *gray legs* has certain geometric relation to the *red* part of the *table* with one *brown top*. by analogy, the *blue* part of the *refrigerator* with *cyan body* has the same geometric to the part of which *color* in the *refrigerator* with *purple body*?

**A:** gray

**Q-type:** geometric\_analogy

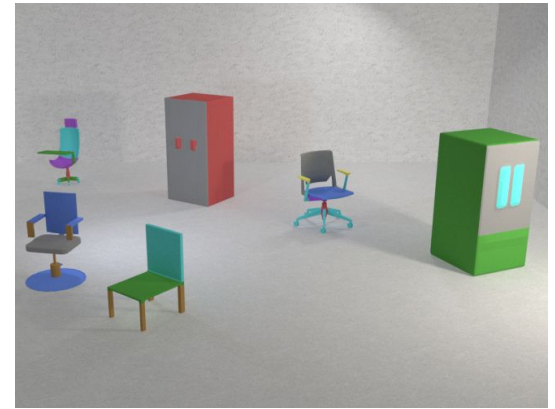

**Q:** The *yellow* parts of the *chair* with *gray back* have certain geometric relation to the *gray* part of the *refrigerator* with *green body*. By analogy, the *brown* parts of the *chair* with *green seat* have the same geometric relation to a part of what *color* in the *chair* with *cyan legs*?

**A:** Blue

**Q-type:** geometric\_analogy

## Arithmetic

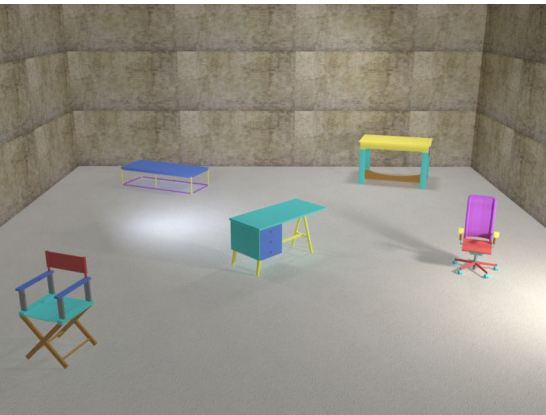

**Q:** What is the sum of the *legs* in the *table* with *blue top*, and the number of *drawers* in the *table* with *cyan top*?

**A:** 9

**Q-type:** sum-minus

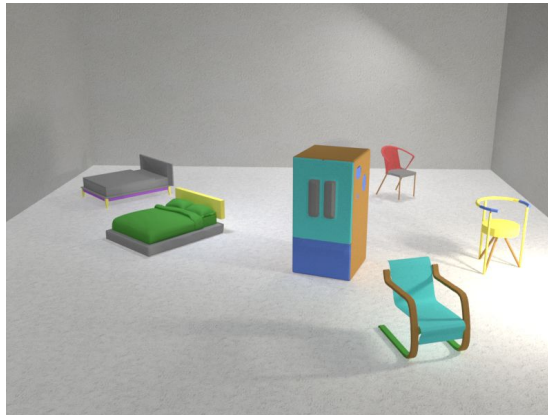

**Q:** Are there an equal number of *doors* in the *refrigerator*, and *leg bars* in the *chair* with *cyan seat*?

**A:** Yes

**Q-type:** compare-integer

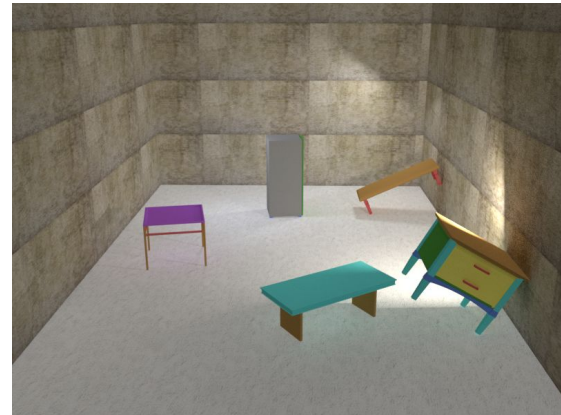

**Q:** Are there fewer *legs* in the *table* with *purple top*, than *drawers* in the *table* with *cyan legs*?

**A:** No

**Q-type:** compare-integer

**Q:** What is the number of *arm vertical bars* in the *chair* with *brown legs*, subtracted by the number of *drawers* in the *table* with *cyan top*?

**A:** 1

**Q-type:** sum-minus

**Q:** Are there fewer *legs* in the *chair* with *gray seat*, than *legs* in the *chair* with *yellow seat*?

**A:** No

**Q-type:** compare-integer

**Q:** What is the number of *drawers* in the *table* with *cyan legs*, subtracted from the number of *legs* in the *table* with *purple top*?

**A:** 2

**Q-type:** sum-minus

# Physics

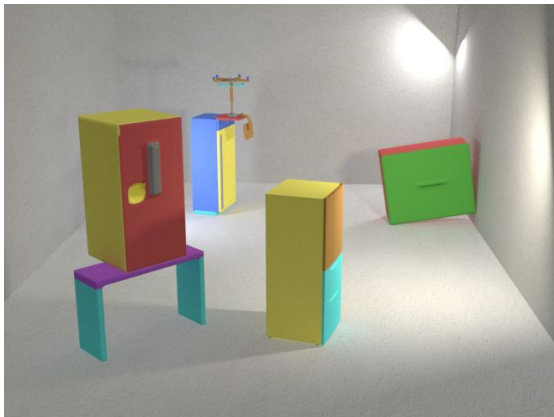

**Q:** Is the *chair* *stable*?

**A:** No

**Q-type:** *stability*

**Q:** Towards which direction should the *chair* move to become *stable*?

**A:** *To left*

**Q-type:** *possible changes*

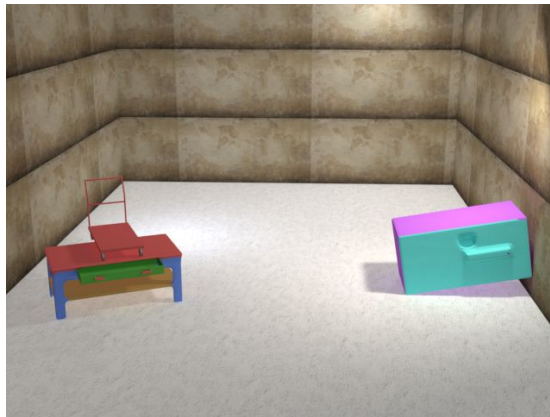

**Q:** How many objects are *stable*?

**A:** 1

**Q-type:** *stability*

**Q:** Can moving *front* makes the *cart* *stable*?

**A:** *no*

**Q-type:** *possible changes*

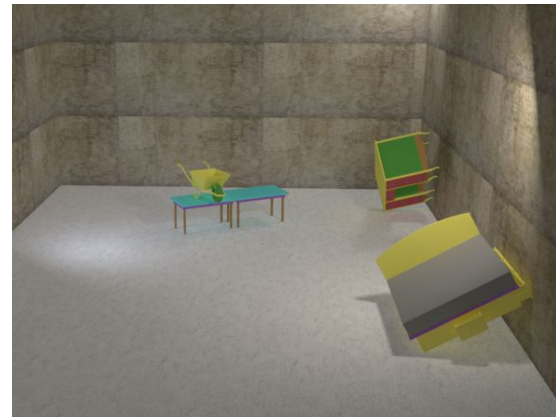

**Q:** Is the *table* with *yellow top* *stable*?

**A:** No

**Q-type:** *stability*

**Q:** Is the *bed* *stable*?

**A:** Yes

**Q-type:** *stability*
